# Supplementary material for: On the Theoretical Properties of the Network Jackknife
Source: arXiv:2004.08935 source file (2020-04-21)
Supplement: Supplementary file 1 [file Supplementary.tex]

\documentclass[11pt]{article}
\usepackage{amsmath,amssymb,amsthm}

\usepackage{graphicx}
\usepackage[table]{xcolor}
\usepackage{bbm}
\usepackage[utf8]{inputenc}
 \usepackage[english]{babel}
 \usepackage{nameref,zref-xr}
 \usepackage[numbers]{natbib}
 \usepackage[pagebackref=true]{hyperref}
% \zxrsetup{toltxlabel}
% \zexternaldocument*{ms_arxiv}
%zexternaldocument*{network_jackknife.tex}
%\renewcommand{\thesubsection}{\Alph{subsection}}
%\renewcommand{\theequation}{\Alph{equation}}
\usepackage{xr}
\externaldocument{network_jackknife}

         % = `top' strut
   % = `bottom' strut

\allowdisplaybreaks

\begin{document}
\input{supplementary_body}

\clearpage
\bibliography{example_paper}
\bibliographystyle{icml2019}

\end{document}
